# Supplementary material for: ATT3D: Amortized Text-to-3D Object Synthesis
Source: arXiv:2306.07349 source file (2023-06-06)
Supplement: Supplementary file 1 [file glossary.tex]

\section{Glossary}\label{sec:app-glossary}
